# Supplementary material for: On the robustness of multimodal language model towards distractions
Source: arXiv:2502.09818 source file (2025-02-13)
Supplement: Supplementary file 1 [file X_suppl.tex]

\clearpage
\setcounter{page}{1}
\maketitlesupplementary

% Add a list of sections in the appendix
\section{Appendix Menu}
\label{sec:appendix}
\begin{itemize}
    \item \hyperref[sec:samples]{Samples}
    \item \hyperref[sec:appendix-statistics]{Statistics of distractions}
    \item \hyperref[sec:appendix-definition]{Definition of distractions}
        \item \hyperref[sec:appendix-more-results]{More Results}
        \item \hyperref[sec:appendix-model-trainingdataset]{Models' training dataset}
\end{itemize}

\newpage
\section{Samples}
\label{sec:samples}

\begin{table*}[h]
\vspace{-0.1in}
\label{tab:samples}
%\vspace{-1.0em}
%\vskip 0.15in
\begin{center}
\small
\begin{tabular}{ccccc}
\toprule
 &\multicolumn{4}{c}{Add Image}  \\
\cmidrule(lr){2-5}&\makecell[c]{\textbf{Neutral Backgrounds}} & \textbf{Generic Landscapes} &\textbf{\makecell[c]{Abstract Art}} &\textbf{\makecell[c]{Everyday Objects}}\\
\makecell[c]{}&\begin{minipage}[b]{0.18\columnwidth}
		\centering
		\raisebox{-.5\height}{\includegraphics[width=\linewidth]{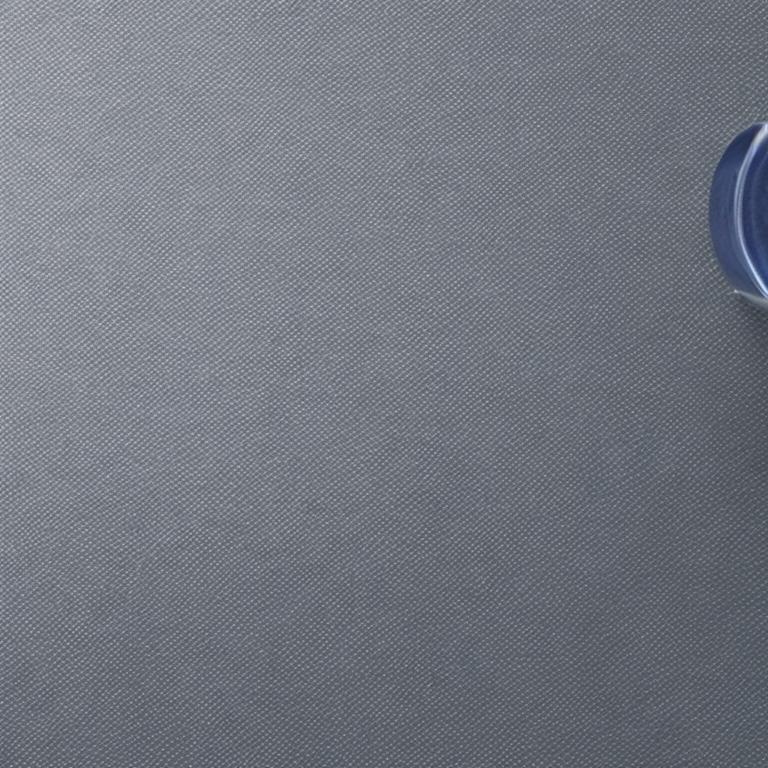}}
	\end{minipage}&\begin{minipage}[b]{0.18\columnwidth}
		\centering
		\raisebox{-.5\height}{\includegraphics[width=\linewidth]{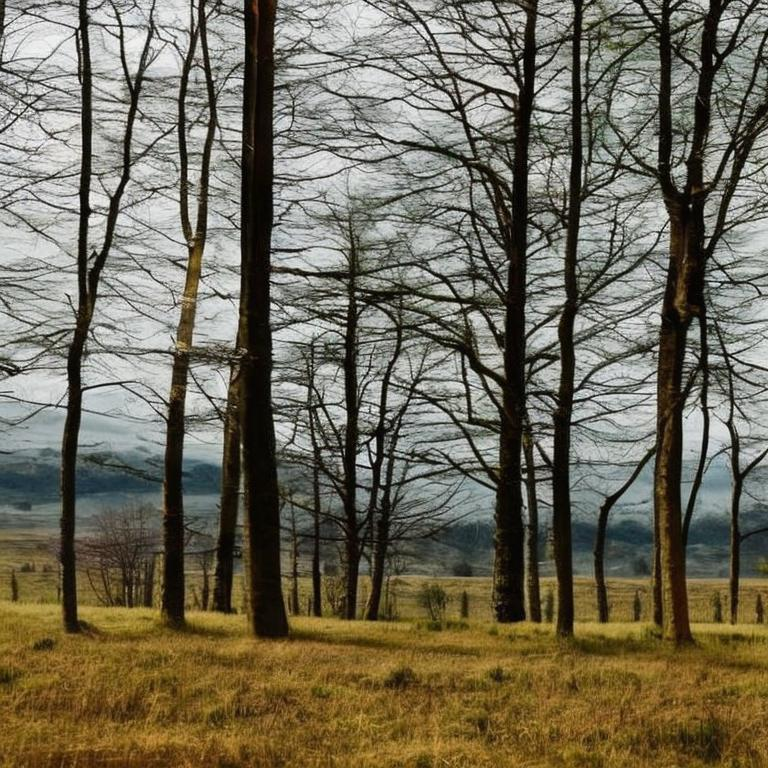}}
	\end{minipage}&\begin{minipage}[b]{0.18\columnwidth}
		\centering
		\raisebox{-.5\height}{\includegraphics[width=\linewidth]{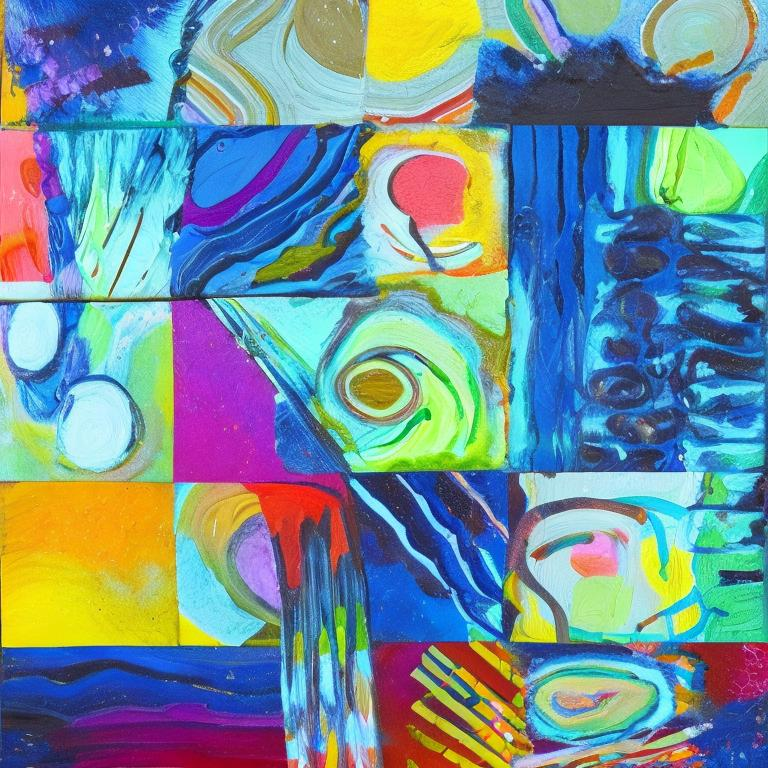}}
	\end{minipage}&\begin{minipage}[b]{0.18\columnwidth}
		\centering
		\raisebox{-.5\height}{\includegraphics[width=\linewidth]{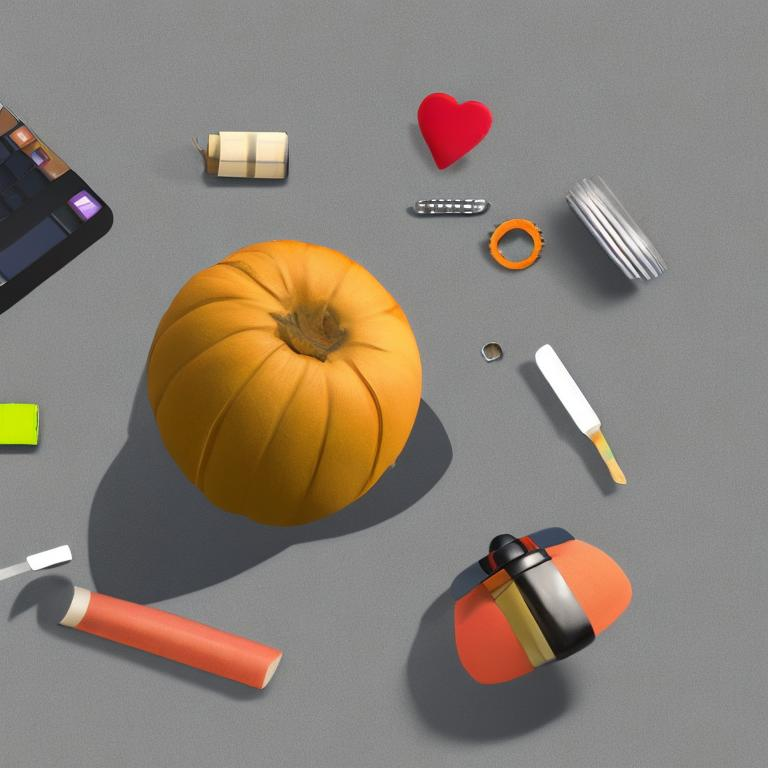}}
	\end{minipage}\\

\cmidrule(lr){2-5}&\textbf{\makecell[c]{Cultural Artifacts}} & \textbf{Emotional Contexts} &\textbf{\makecell[c]{Digital Creations}} &\textbf{\makecell[c]{Word Embeddings}}\\
\makecell[c]{}&\begin{minipage}[b]{0.18\columnwidth}
		\centering
		\raisebox{-.5\height}{\includegraphics[width=\linewidth]{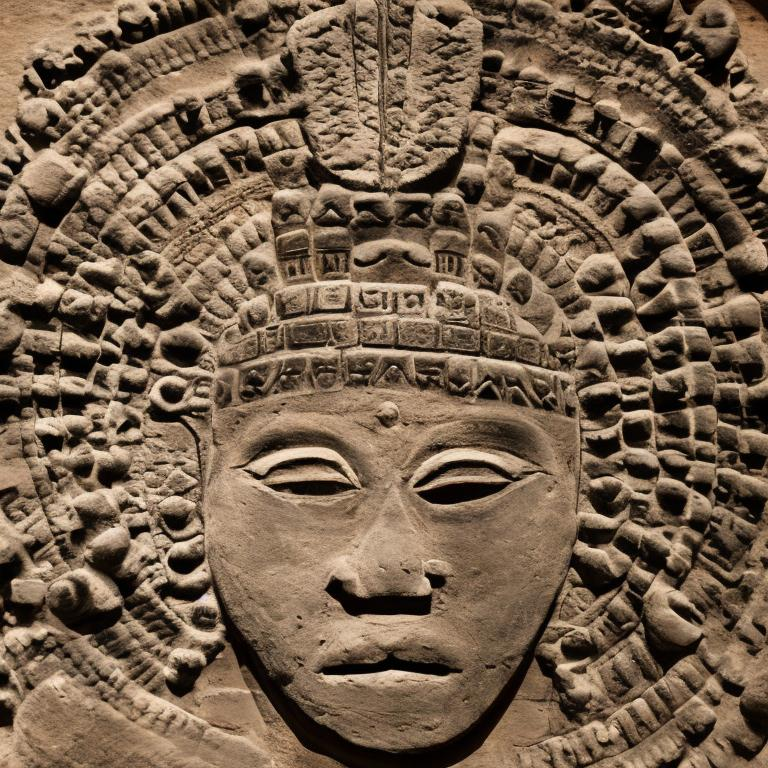}}
	\end{minipage}&\begin{minipage}[b]{0.18\columnwidth}
		\centering
		\raisebox{-.5\height}{\includegraphics[width=\linewidth]{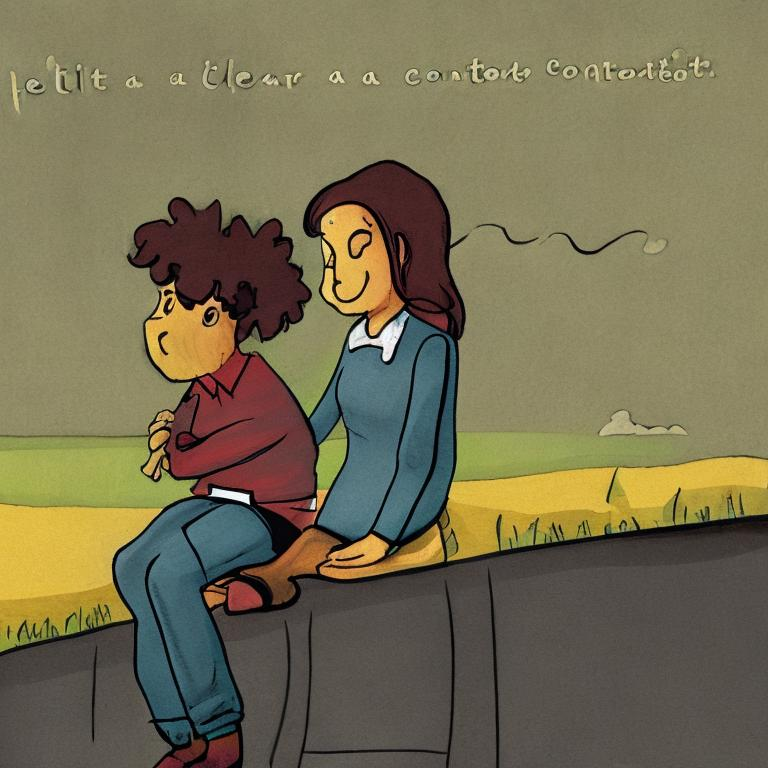}}
	\end{minipage}&\begin{minipage}[b]{0.18\columnwidth}
		\centering
		\raisebox{-.5\height}{\includegraphics[width=\linewidth]{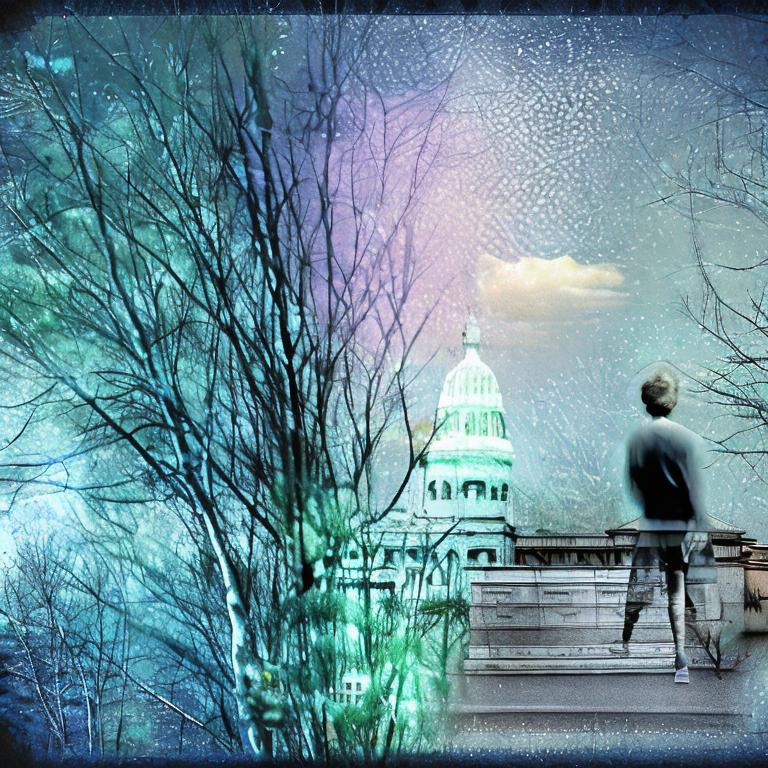}}
	\end{minipage}&\begin{minipage}[b]{0.18\columnwidth}
		\centering
		\raisebox{-.5\height}{\includegraphics[width=\linewidth]{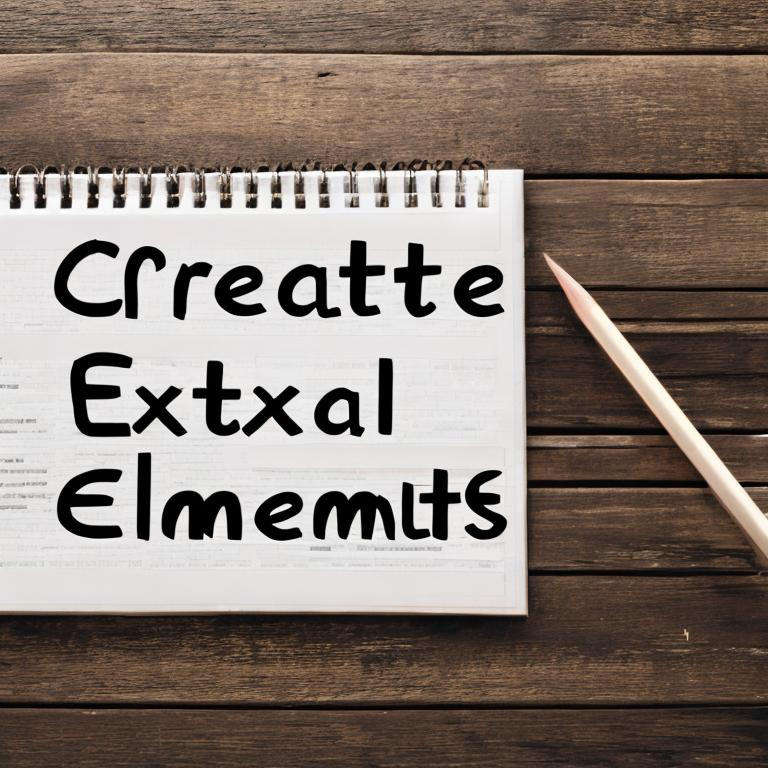}}
	\end{minipage}\\
\midrule
&\multicolumn{4}{c}{Add Hint}  \\

\cmidrule(lr){2-5}&\textbf{\makecell[c]{Non \\Sequitur}} & \textbf{\makecell[c]{Contradictory \\Information}} &\makecell[c]{\textbf{\makecell[c]{Irrelevant\\Information}}} &\makecell[c]{\textbf{\makecell[c]{Misleading \\Information}}} \\
\makecell[c]{} & \makecell[c]{Bananas are yellow, and \\I have never been to\\ Antarctica.} & \makecell[c]{Chocolate is actually \\a vegetable.} &\makecell[c]{Bananas are berries, \\but strawberries are not.} &\makecell[c]{That vaccines \\cause autism.} \\
\bottomrule
\end{tabular}
\end{center}
\caption{Examples of various distraction subtypes within the \textbf{Add Image} and \textbf{Add Hint} scenarios of our \emph{I-ScienceQA} benchmark, derived from the \emph{ScienceQA} dataset~\citep{lu2022scienceqa}.}
\end{table*}

\section{Statistics of distractions}
\label{sec:appendix-statistics}

\begin{table*}[h]
    \centering
    \begin{tabular}{p{2.5cm}p{7cm}c}
        \toprule
        \textbf{Scenario} & \textbf{Types of Distraction and Content} & \textbf{Number} \\
        \midrule
        \multirow{8}{*}{Add Image} 
            & Neutral Backgrounds & 250 \\ 
            & Generic Landscapes & 250 \\ 
            & Abstract Art & 250 \\ 
            & Everyday Objects & 250 \\ 
            & Cultural Artifacts & 250 \\ 
            & Digital Creations & 250 \\ 
            & Word Embeddings & 250 \\ 
            & Emotional Contexts & 250 \\ 
        \midrule
        \multirow{9}{*}{Insert Image}
            & Diffusion Inpainting & 100 \\
            & Neutral Backgrounds & 250 \\ 
            & Generic Landscapes & 250 \\ 
            & Abstract Art & 250 \\ 
            & Everyday Objects & 250 \\ 
            & Cultural Artifacts & 250 \\ 
            & Digital Creations & 250 \\ 
            & Word Embeddings & 250 \\ 
            & Emotional Contexts & 250 \\ 
        \midrule
        \multirow{5}{*}{Add Hints} 
            & Irrelevant Context Integration & 400 \\ 
            & Contradictory Information & 400 \\ 
            & Non Sequitur & 400 \\ 
            & Misleading Information & 400 \\ 
            & Ambiguous Information & 400 \\ 
        \midrule
        \multirow{5}{*}{Insert Hints} 
            & Subtle Misinformation & 400 \\ 
            & Irrelevant Details & 400 \\ 
            & Disruptive Narrative Inserts & 400 \\ 
            & Complex Referential Distractions & 400 \\ 
            & Ambiguous Information & 400 \\ 
        \bottomrule
    \end{tabular}
    \caption{Distribution of Distraction Scenarios Across Scenarios}
    \label{tab:dataset statistics}
\end{table*}

\section{Definition for distractions}
\label{sec:appendix-definition}

\begin{table*}[H]
\centering
\begin{tabular}{p{3cm}p{9cm}}
\toprule
\textbf{Type of Image} & \textbf{Description} \\
\midrule
Neutral Backgrounds & Simple, monochromatic backgrounds to minimize distraction and control variable introduction. \\
\midrule
Generic Landscapes & Broad, non-specific landscapes (e.g., forests, urban scenes, mountains) that provide a realistic yet contextually neutral backdrop. \\
\midrule
Abstract Art & Non-representational art that challenges the model to focus on textual rather than visual cues. \\
\midrule
Everyday Objects & Common, non-contextual objects to evaluate the model's ability to disregard irrelevant visual stimuli. \\
\midrule
Cultural Artifacts & Images of artifacts that test cultural recognition and contextual integration capabilities. \\
\midrule
Digital Creations & Computer-generated or altered imagery to assess the model's response to unconventional visual data. \\
\midrule
Word Embeddings & Images with embedded or overlaid text to examine effective textual and visual information merging. \\
\midrule
Emotional Contexts & Images depicting clear emotional tones to probe model's alignment of text and visual emotion cues. \\
\bottomrule
\end{tabular}
\caption{Types and definition of Distractions for Scenario I \textbf{Add Image} and Scenario II \textbf{Insert Image}.}
\label{tab:definition add images}
\end{table*}

\begin{table*}[h]
\centering
\begin{tabular}{p{3cm}p{9cm}}
\toprule
\textbf{Type of Image} & \textbf{Description} \\
\midrule
Flying Objects & Introduces elements like birds, planes, or insects, requiring the model to differentiate between essential static elements and moving distractions. \\
\midrule
Floating Balloons & Adds balloons of various colors and sizes that float across the scene, testing the VLM's ability to ignore appealing but irrelevant moving objects. \\
\midrule
Passing Vehicles & Populates scenes with moving vehicles like cars and bicycles, challenging the model to disregard transient elements. \\
\midrule
Drifting Clouds & Simulates clouds moving across the sky, testing the model's focus amid ongoing environmental changes. \\
\midrule
Bouncing Balls & Uses images of balls in motion to introduce unexpected kinetic elements, assessing the model's response to sudden movements. \\
\midrule
Swarming Insects & Adds complexity with swarming insects like butterflies or bees to test the VLM's fine-grained visual attention. \\
\midrule
Animated Signs & Integrates changing digital signs to evaluate the model's ability to ignore intermittent visual stimuli. \\
\midrule
Symbols and Icons & Embeds non-contextual symbols or icons, assessing the model's disregard for extraneous visual information. \\
\midrule
Overlaid Words & Overlays random words or phrases to introduce visual clutter, testing prioritization of primary textual content. \\
\midrule
Sitting Pets & Includes images of sitting pets to test the VLM's focus amidst visually appealing but irrelevant elements. \\
\bottomrule
\end{tabular}
\caption{Types and definition of Distractions for Scenario II: \textbf{Insert Image}.}
\label{tab:defintition insert image}
\end{table*}

\begin{table*}[h]
\centering
\begin{tabular}{p{3.5cm}p{8.5cm}}
\toprule
\textbf{Distraction Type} & \textbf{Description} \\
\midrule
Irrelevant Context Integration & Introduce sentences with contextually irrelevant information to assess the model's capacity to filter out noise. Based on studies showing extraneous data can reduce comprehension accuracy, mirroring real-world information processing challenges. \\
\midrule
Contradictory Information & Embed contradictions within the narrative to test the models' conflict resolution and logic adherence capabilities. \\
\midrule
Non Sequitur & Use complex sentence structures and ambiguous phrases to evaluate the models' parsing and interpretation flexibility. \\
\midrule
Misleading Information & Include plausible but incorrect data points within texts, testing the models' fact-checking abilities and resilience against misinformation. \\
\midrule
Ambiguous Information & Incorporate vague or unclear statements to assess the model's ability to handle uncertainty and make reasonable inferences. \\
\bottomrule
\end{tabular}
\caption{Types and definition of Distractions for Scenario III: \textbf{Add Hint}.}
\label{tab:definition add hints}
\end{table*}

\begin{table*}[h]
\centering
\small
\begin{tabular}{>{\raggedright\arraybackslash}p{0.25\textwidth}|>{\raggedright\arraybackslash}p{0.65\textwidth}}
\toprule
\textbf{Distraction Type} & \textbf{Description} \\
\midrule
Subtle Misinformation & Inserts information that subtly misleads, contradicting established data yet remaining plausible within the context. \\
\midrule
Irrelevant Details & Introduces extraneous details that do not contribute to the task, challenging the model to maintain focus on relevant content. \\
\midrule
Disruptive Narrative Inserts & Incorporates unrelated narratives that interrupt logical progression, testing the model's information filtering capabilities. \\
\midrule
Complex Referential Distractions & Utilizes intricate language and referential sequences that complicate the parsing process, assessing interpretative accuracy. \\
\midrule
Ambiguous or Conflicting Information & Presents choices that include both plausible and incorrect answers, exploiting potential ambiguities to test decision-making precision. \\
\bottomrule
\end{tabular}
\caption{Types and definition of Distractions for Scenario IV: \textbf{Insert Hint}.}
\label{tab:definition insert hints}
\end{table*}

\section{More results}
\label{sec:appendix-more-results}

\subsection{Add Image}
\begin{table*}[H]
  \centering
  \caption{Exact Match Scores of Various Models Across Different Types of Distractions in the \textbf{Add Image} Scenario. Abbreviations: AA = Abstract Art, CA = Cultural Artifacts, WE = Word Embeddings, DC = Digital Creations, NB = Neutral Backgrounds, GL = Generic Landscapes, EC = Emotional Contexts, EO = Everyday Objects.}
  \label{tab:performance_metrics_details_add_image}
  \sisetup{
    table-number-alignment = center,
    round-mode = places,
    round-precision = 1
  }
  \begin{tabular}{l *{8}{S[table-format=2.1]}}
    \toprule
    \textbf{Model} & \textbf{AA} & \textbf{CA} & \textbf{WE} & \textbf{DC} & \textbf{NB} & \textbf{GL} & \textbf{EC} & \textbf{EO} \\
    \midrule
    InstructBLIP (7B)             & 38.8 & 37.6 & 44.4 & 42.4 & 37.6 & 42.4 & 40.0 & 45.2 \\
    InstructBLIP (13B)            & 70.4 & 72.0 & 73.6 & 75.2 & 73.2 & 70.4 & 67.6 & 73.6 \\
    Llava (7B)                    & 66.4 & 73.2 & 71.6 & 70.8 & 64.4 & 69.6 & 62.8 & 65.6 \\
    Llava (13B)                   & 70.4 & 72.0 & 73.6 & 75.2 & 73.2 & 70.4 & 67.6 & 73.6 \\
    Internvl2 (2B)                & 83.6 & 84.4 & 85.6 & 87.2 & 92.4 & 88.0 & 86.8 & 86.0 \\
    Internvl2 (8B)                & 94.8 & 96.0 & 93.6 & 95.6 & 93.6 & 93.6 & 92.0 & 96.4 \\
    Qwen/Qwen2-VL-2B-Instruct      & 59.6 & 63.6 & 60.0 & 64.0 & 67.6 & 63.2 & 65.2 & 63.2 \\
    Qwen/Qwen2-VL-7B-Instruct      & 84.8 & 82.0 & 83.2 & 85.6 & 81.6 & 84.4 & 83.2 & 80.0 \\
    THUDM/cogVLM2-LLaMA3-Chat-19B & 69.2 & 72.8 & 72.0 & 70.8 & 73.2 & 74.4 & 69.2 & 72.4 \\
     GPT-4o                       & 94.0 & 94.0 & 90.8 & 92.0 & 91.2 & 94.0 & 94.8 & 93.2 \\
    \bottomrule
  \end{tabular}
\end{table*}

\subsection{Insert Image}

\begin{table*}[H]
  \centering
  \caption{Exact Match Scores of Various Models Across Different Types of Distractions in the \textbf{Insert Image} Scenario. Abbreviations: AA = Abstract Art, CA = Cultural Artifacts, WE = Word Embeddings, DC = Digital Creations, NB = Neutral Backgrounds, GL = Generic Landscapes, EC = Emotional Contexts, EO = Everyday Objects, DI = Diffusion Inpainting.}
  \label{tab:performance_metrics_details_insert_image}
  \sisetup{
    table-number-alignment = center,
    round-mode = places,
    round-precision = 2
  }
  \begin{tabular}{l *{9}{S[table-format=2.2]}}
    \toprule
    \textbf{Model} & \textbf{AA} & \textbf{CA} & \textbf{WE} & \textbf{DC} & \textbf{NB} & \textbf{GL} & \textbf{EC} & \textbf{EO} & \textbf{DI} \\
    \midrule
    InstructBLIP (7B)             & 32.40 & 39.20 & 34.00 & 34.40 & 37.60 & 36.80 & 36.00 & 30.40 & 42.42 \\
    InstructBLIP (13B)            & 68.80 & 72.00 & 69.60 & 70.80 & 73.20 & 68.40 & 66.80 & 66.00 & 72.73 \\
    Llava (7B)                    & 63.60 & 70.80 & 67.60 & 67.20 & 68.80 & 68.40 & 60.40 & 64.80 & 64.64 \\
    Llava (13B)                   & 68.80 & 72.00 & 69.60 & 70.80 & 73.20 & 68.40 & 66.80 & 66.00 & 72.72 \\
    Internvl2 (2B)                & 89.20 & 87.20 & 91.20 & 91.20 & 91.20 & 92.00 & 90.80 & 90.00 & 87.87 \\
    Internvl2 (8B)                & 94.00 & 92.40 & 93.60 & 94.80 & 95.60 & 96.00 & 95.20 & 93.60 & 90.90 \\
    Qwen/Qwen2-VL-2B-Instruct      & 62.40 & 64.80 & 64.40 & 68.00 & 64.40 & 67.20 & 60.40 & 58.80 & 52.53 \\
    Qwen/Qwen2-VL-7B-Instruct      & 64.40 & 70.80 & 68.00 & 71.20 & 72.00 & 70.40 & 61.60 & 68.80 & 61.62 \\
    THUDM/cogVLM2-LLaMA3-Chat-19B & 89.20 & 86.80 & 86.00 & 87.60 & 87.20 & 89.20 & 86.80 & 88.00 & 84.85 \\
     GPT-4o                       & 79.60 & 79.60 & 78.00 & 82.00 & 78.80 & 78.00 & 77.20 & 76.40 & 75.75 \\
    \bottomrule
  \end{tabular}
\end{table*}

\subsection{Add Hint}

\begin{table*}[h!]
  \centering
  \caption{Exact Match Scores of Various Models Across Different Types of Distractions in the \textbf{Add Hint} Scenario. Abbreviations: Contradictory = Contradictory Hints, Non Sequitur = Non Sequitur Hints, Ambiguous = Ambiguous Hints, Irrelevant = Irrelevant Hints, Misleading = Misleading Hints.}
  \label{tab:performance_metrics_details_add_hint}
  \sisetup{
    table-number-alignment = center,
    round-mode = places,
    round-precision = 2
  }
  \begin{tabular}{l *{5}{S[table-format=2.2]}}
    \toprule
    \textbf{Model} & \textbf{Contradictory} & \textbf{Non Sequitur} & \textbf{Ambiguous} & \textbf{Irrelevant} & \textbf{Misleading} \\
    \midrule
    InstructBLIP (7B)                      & 62.75 & 65.00 & 66.50 & 58.75 & 66.00 \\
    InstructBLIP (13B)                     & 67.50 & 69.25 & 68.00 & 63.75 & 68.75 \\
    Llava (7B)                             & 63.60 & 70.80 & 67.60 & 67.20 & 68.80 \\
    Llava (13B)                            & 68.80 & 72.00 & 69.60 & 70.80 & 73.20 \\
    Internvl2 (2B)                         & 81.50 & 77.00 & 87.00 & 85.75 & 80.50 \\
    Internvl2 (8B)                         & 95.00 & 92.00 & 94.50 & 92.25 & 94.25 \\
    Qwen/Qwen2-VL-2B-Instruct               & 53.00 & 55.00 & 59.25 & 52.00 & 53.00 \\
    Qwen/Qwen2-VL-7B-Instruct               & 67.75 & 68.25 & 71.75 & 67.50 & 64.75 \\
    THUDM/cogVLM2-LLaMA3-Chat-19B          & 74.50 & 68.25 & 73.75 & 68.00 & 68.00 \\
     GPT-4o                                 & 90.00 & 87.50 & 87.50 & 84.75 & 87.75 \\
    \bottomrule
  \end{tabular}
\end{table*}

\begin{table*}[ht]
  \centering
  \caption{Exact Match Scores of Various Models Across Different Types of Distractions in the \textbf{Insert Hint} Scenario. Abbreviations: Subtle Misinformation = Influence of Subtle Misinformation Hints, Irrelevant Details = Influence of Irrelevant Details Hints, Disruptive Narrative = Influence of Disruptive Narrative Hints, Complex Referential = Influence of Complex Referential Hints, Ambiguous or Conflicting = Influence of Ambiguous or Conflicting Hints.}
  \label{tab:performance_metrics_details_insert_hint}
  \begin{adjustbox}{max width=\textwidth}
    \sisetup{
      table-number-alignment = center,
      round-mode = places,
      round-precision = 2
    }
    \begin{tabular}{l *{5}{S[table-format=2.2]}}
      \toprule
      \textbf{Model} & \textbf{Subtle Misinformation} & \textbf{Irrelevant Details} & \textbf{Disruptive Narrative} & \textbf{Complex Referential} & \textbf{Ambiguous or Conflicting} \\
      \midrule
      Llava (7B)                             & 70.75 & 69.50 & 67.50 & 69.75 & 69.00 \\
      Llava (13B)                            & 74.00 & 73.50 & 70.00 & 70.50 & 71.00 \\
      Internvl2 (2B)                         & 90.25 & 92.25 & 90.50 & 93.75 & 90.75 \\
      Internvl2 (8B)                         & 95.00 & 95.75 & 94.25 & 97.25 & 97.25 \\
       Qwen/Qwen2-VL-2B-Instruct    & 65.75 & 65.00 & 59.75 & 66.00 & 64.50 \\
      Qwen/Qwen2-VL-7B-Instruct    & 76.00 & 71.75 & 73.25 & 74.25 & 75.25 \\
      THUDM/cogVLM2-LLaMA3-Chat-19B & 78.75 & 79.25 & 81.75 & 83.50 & 81.00 \\
       GPT-4o                                 & 83.75 & 84.75 & 83.00 & 82.25 & 86.50 \\
      \bottomrule
    \end{tabular}
  \end{adjustbox}
\end{table*}

\clearpage
\onecolumn
\section{Models' training dataset}
\label{sec:appendix-model-trainingdataset}

\begin{longtable}{|l|p{10cm}|}
\hline
\textbf{Model Name} & \textbf{Training Data} \\
\hline
\endfirsthead

\hline
\textbf{Model Name} & \textbf{Training Data} \\
\hline
\endhead

\hline
\endfoot

\hline
\endlastfoot

\multirow{2}{*}{liu2023llava1.5} & 
\textbf{Pre-training data:} Conceptual Captions (CC) \citep{changpinyo2021conceptual}; COCO Captions \citep{lin2014microsoft}; ScienceQA \citep{lu2022scienceqa}; LLaVA-Instruct-158K \citep{liu2023llava}; utilizes a CLIP visual encoder pre-trained on LAION-2B \citep{schuhmann2022laion}. \\
& 
\textbf{Fine-tuning data:} COCO \citep{lin2014microsoft}; ScienceQA \citep{lu2022scienceqa}; LLaVA-Instruct-158K \citep{liu2023llava}, tailored for instruction-following tasks. \\
\hline
\multirow{2}{*}{InstructBLIP-Vicuna (7B, 13B)} & 
\textbf{Pre-training data:} NoCaps \citep{nocaps}; Flickr30K \citep{flickr30k}; VizWiz \citep{vizwiz}; GQA \citep{hudson2019gqa}; Visual Spatial Reasoning \citep{liu2023vsr}; IconQA \citep{iconqa}; ScienceQA \citep{lu2022scienceqa}; Visual Dialog \citep{das2017visualdialog}; TextVQA \citep{singh2019towards}; HatefulMemes \citep{hatefulmemes}; MSVD-QA \citep{msvdqa}; MSRVTT-QA \citep{msrvttqa}; iVQA \citep{ivqa}. \\
& 
\textbf{Fine-tuning data:} COCO Caption \citep{lin2014microsoft}; Web CapFilt \citep{li2022blip, li2022blip}; TextCaps \citep{sidorov2020textcaps}; VQAv2 \citep{goyal2017vqav2}; OKVQA \citep{marino2019okvqa}; A-OKVQA \citep{schwenk2022aokvqa}; OCR-VQA \citep{mishra2019ocrvqa}; LLaVA-Instruct-150K \citep{liu2023llava}, transformed into instruction-answer pairs for enhanced multimodal instruction following. \\
\hline
\multirow{2}{*}{CogVLM2-LLaMA3-Chat-19B} & 
\textbf{Pre-training data:} LAION-2B \citep{schuhmann2022laion}; COYO-700M \citep{byeon2022coyo}; LAION-40M-grounding \citep{zhang2022glipv2}; multilingual image-text pairs from LAION, COCO \citep{lin2014microsoft}, and Visual Genome \citep{visualgenome}. \\
& 
\textbf{Fine-tuning data:} OKVQA \citep{marino2019okvqa}; STVQA \citep{biten2019stvqa}; visualgenome \citep{visualgenome}; VQAv2 \citep{goyal2017vqav2}; DocVQA \citep{mathew2021docvqa}; OCRVQA \citep{mishra2019ocrvqa}; TextVQA \citep{singh2019towards}; GeoMetry3K \citep{lu2021inter}; Geo170K \citep{Geo170K}; GeoQA \citep{GeoQA}; ScienceQA \citep{lu2022scienceqa}; ChartQA \citep{masry2022chartqa}; FigureVQA \citep{FigureQA}; InfoVQA \citep{mathew2022infographicvqa}; DVQA \citep{kafle2018dvqa}; ArxivQA \citep{ArxivQA}; TDIUC \citep{TDIUC}; TallyQA \citep{TallyQA}, optimized for multimodal understanding and conversational abilities. \\
\hline
\multirow{2}{*}{Qwen2-VL-7B-Instruct} & 
\textbf{Pre-training data:} Details not publicly disclosed. \\
& 
\textbf{Fine-tuning data:} Details not publicly disclosed. \\
\hline
\multirow{2}{*}{Phi3-V} & 
\textbf{Pre-training data:} Details not publicly disclosed. \\
& 
\textbf{Fine-tuning data:} Details not publicly disclosed. \\
\hline
\pagebreak % Forces a page break here
\multirow{2}{*}{InternVL2 (2B, 8B)} & 
\textbf{Pre-training data:} Laion-EN \citep{schuhmann2022laion}; Laion-ZH (zh) \citep{schuhmann2022laion}; COYO (zh) \citep{byeon2022coyo}; GRIT (zh) \citep{peng2023kosmos2}; COCO \citep{lin2014microsoft}; TextCaps \citep{sidorov2020textcaps}; Objects365 (en\&zh) \citep{shao2019objects365}; GRIT (en\&zh) \citep{peng2023kosmos2}; All-Seeing (en\&zh) \citep{wang2023allseeing}; Wukong-OCR (zh) \citep{gu2022wukong}; LaionCOCO-OCR \citep{schuhmann2022laioncoco}; MMC-Inst \citep{liu2023mmcinst}; LSVT (zh) \citep{sun2019lsvt}; ST-VQA \citep{biten2019stvqa}; RCTW-17 (zh) \citep{shi2017rctw17}; ReCTs (zh) \citep{zhang2019rects}; ArT (en\&zh) \citep{chng2019art}; SynthDoG (en\&zh) \citep{kim2022synthdog}; COCO-Text \citep{veit2016cocotext}; ChartQA \citep{masry2022chartqa}; CTW (zh) \citep{yuan2019ctw}; DocVQA \citep{mathew2021docvqa}; TextOCR \citep{singh2021textocr}; PlotQA \citep{methani2020plotqa}; InfoVQA \citep{mathew2022infographicvqa}. \\
& 
\textbf{Fine-tuning data:} TextCaps \citep{sidorov2020textcaps}; ShareGPT4V (en\&zh) \citep{chen2023sharegpt4v}; VQAv2 \citep{goyal2017vqav2}; GQA \citep{hudson2019gqa}; OKVQA \citep{marino2019okvqa}; VSR \citep{liu2023vsr}; Visual Dialog \citep{das2017visualdialog}; AI2D \citep{kembhavi2016ai2d}; ScienceQA \citep{lu2022scienceqa}; TQA \citep{kembhavi2017tqa}; ChartQA \citep{masry2022chartqa}; MMC-Inst \citep{liu2023mmcinst}; DVQA \citep{kafle2018dvqa}; PlotQA \citep{methani2020plotqa}; GeoQA+ \citep{cao2022geoqa_plus}; TabMWP \citep{lu2022tablemwp}; MathQA \citep{yu2023mathqa}; CLEVR-Math/Super \citep{lindstrom2022clevrmath, li2023superclevr}; Geometry3K \citep{lu2021inter}; KVQA \citep{shah2019kvqa}; A-OKVQA \citep{schwenk2022aokvqa}; ViQuAE \citep{lerner2022viquae}; Wikipedia (en\&zh) \citep{he2023wanjuan}; OCRVQA \citep{mishra2019ocrvqa}; TextVQA \citep{singh2019towards}; RefCOCO/+/g \citep{yu2016refcoco, mao2016refcocog}; Visual Genome \citep{visualgenome}; LLaVA-1580K (en\&zh) \citep{liu2023llava}; LVIS-Instruct4V \citep{wang2023lvisinstruct4v}; ALLaVA (en\&zh) \citep{chen2024allava}; Laion-GPT4V \citep{laion_gpt4v_dataset}; TextOCR-GPT4V \citep{textocr_gpt4v_dataset}; SVIT (en\&zh) \citep{zhao2023svit}; OpenHermes2.5 \citep{OpenHermes2_5}; Alpaca-GPT4 \citep{taori2023alpaca}; ShareGPT (en\&zh) \citep{zheng2023vicuna}; COIG-CQIA (zh) \citep{bai2024coig}; optimized for diverse visual-language tasks including visual question answering, image captioning, and visual dialogue. \\
\hline
\multirow{2}{*}{GPT-4o} & 
\textbf{Pre-training data:} Details not publicly disclosed. \\
& 
\textbf{Fine-tuning data:} Details not publicly disclosed. \\
\hline
\caption{Models and their Pre-training and Fine-tuning Data}
\end{longtable}
\label{tab:training_data_long}
\clearpage
\twocolumn
